# Supplementary material for: DiSPy: Implementation of Distortion Symmetry for the Nudged Elastic Band Method
Source: arXiv:1810.01911 ancillary file (2018-12-20)
Supplement: Supplementary file 1 [file supplementary.pdf]

# SUPPLEMENTARY MATERIAL

## Supplementary Note 1: Irreducible representations.

The elements of a mathematical group $s \in S$ can be represented on a vector space $V$ through a mapping of $s$ to a linear transformation in $V$ given by the matrix $D(s)$. In general, the representation $D$ (the set $\{D(s)\}$) of any finite group can be decomposed into a linear combination of its $n$ irreducible representations (irreps)[1]:

$$D = c_1\Gamma_1 \oplus c_2\Gamma_2 \oplus \dots\ c_n\Gamma_n. \tag{1}$$

Here, $c_i$ are positive integers, and $\Gamma_i$ are the irreps. In other words, the matrix $D(s)$ representing element $s$ in some finite crystallographic group $S$ can be written as

$$D(s) = \begin{bmatrix} \Gamma_1(s) & 0 & \dots & 0 \\ 0 & \Gamma_2(s) & \dots & 0 \\ & & \ddots & \\ 0 & 0 & & 0 \\ 0 & 0 & \dots & \Gamma_n(s) \end{bmatrix} \tag{2}$$

where the $\Gamma_i(s)$ matrix will appear $c_i$ times along the diagonal. Consequently, the irrep matrices of a group may be found by choosing a reducible representation $(D')$ containing all $n$-irreps, and determining a matrix $T$ such that

$$D(s) = T^{-1}D'(s)T,\ \forall s \in S. \tag{3}$$

It should be noted that one can directly calculate the $c_i$ coefficients given matrices that form a reducible representation, and the character table for a given finite group [1]:

$$c_i = \frac{1}{h}\sum_{s\in S}\chi_i(s)\chi'(s), \tag{4}$$

where $h$ is the order of the group, $\chi_i(s)$ is the trace of the marix representing $s$ in the $i$th irrep, and $\chi'(s)$ is the trace of the matrix representing $s$ in the reducible representation $D'$. It should be noted that elements within the same conjugacy classes will have the same trace, and will therefore result in duplicate entries in the sum in Eq. 4 which still need to be included.

By constructing $D'$ using a vector space of quantities such as atomic displacements, the eigenvectors of $T$ will provide displacive vectors which will transform as the irreps of $S$, and have the symmetry of their kernels. This corresponds to the set of all elements which map to identity in a given irrep. However, for a crystallographic space group $S$ that has an infinite number of unit spatial translations, irreps must also consider a wave vector $\mathbf{b}$ in the first Brillouin zone [1]. By applying the above procedure when the set $\{s\}$ is chosen to be the coset representatives of the group of $T_g$ in $S$, where $T_g$ is the group of all unit translations, irrep matrices at $\Gamma$ [$\mathbf{b} = (0, 0, 0)$] are generated. More generally, the matrices for irreps at other $\mathbf{b}$ vectors can be determined by considering the group of the wave vector $S^k$. This is the group of all $s \in G$ such that

$$s\mathbf{b} = \mathbf{b}R^{-1} = \mathbf{b}\ (\text{mod}\ \mathbf{B}), \tag{5}$$

where $R$ is the rotational part of the matrix-vector pair representing $s$, and $\mathbf{B}$ is a reciprocal-lattice vector. Using this group, the irrep matrices can be generated using a well-established induction procedure. For more detailed information about this, see Ref. [1, 2].

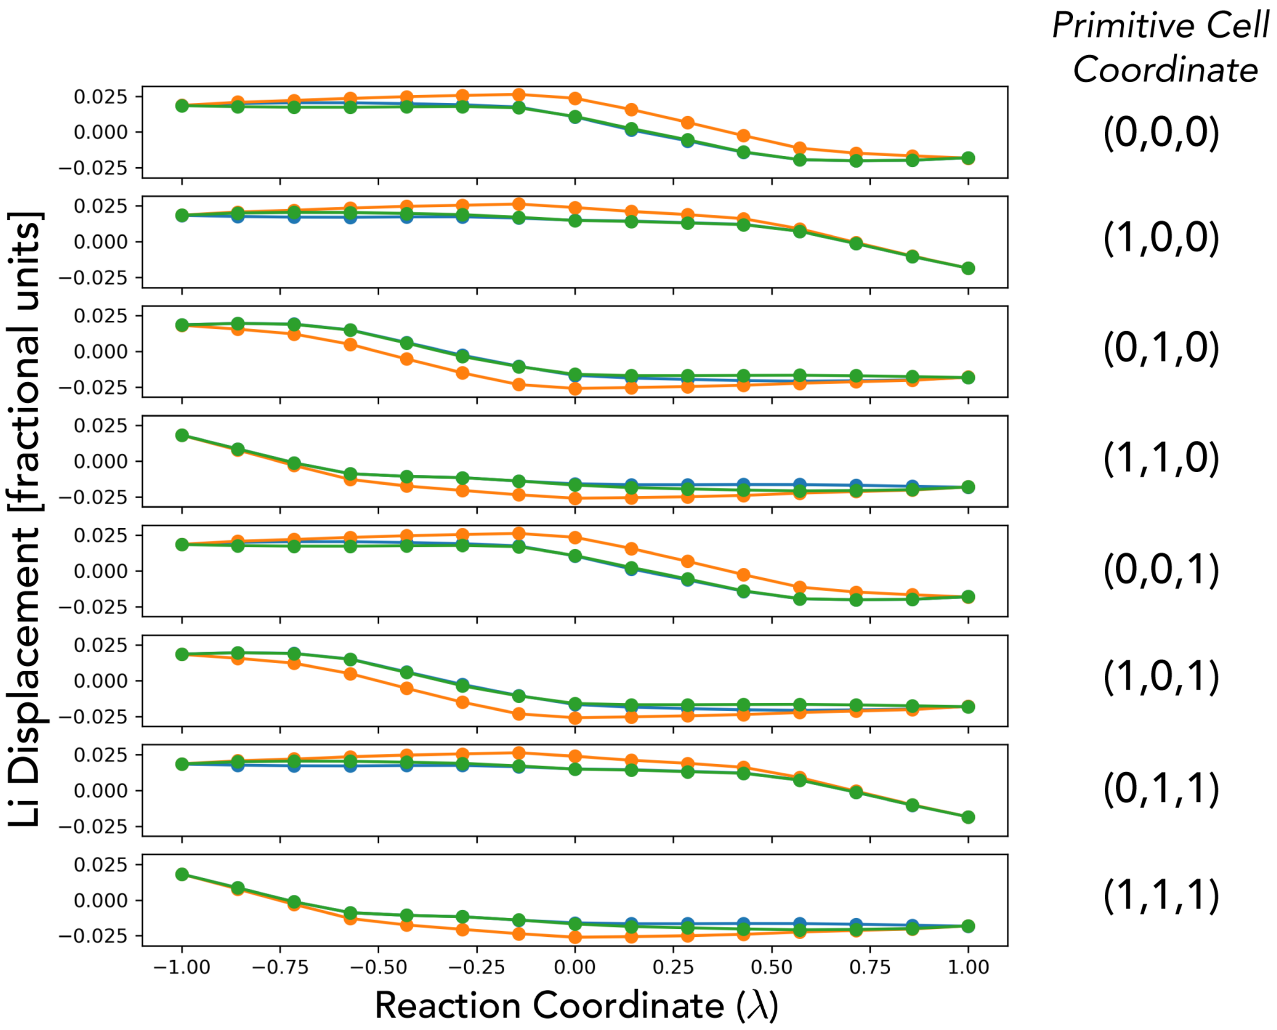


**Supplementary Figure 1.** Plot of the displacement of both Li atoms within each primitive rhombohedral unit cell along each of the cell vectors in Fig. 5a as a function of reaction coordinate. Data is plotted for the path with $P1$ symmetry shown in red in Fig. 5b. The high-symmetry structure with $R\bar{3}c$ symmetry is taken as reference.

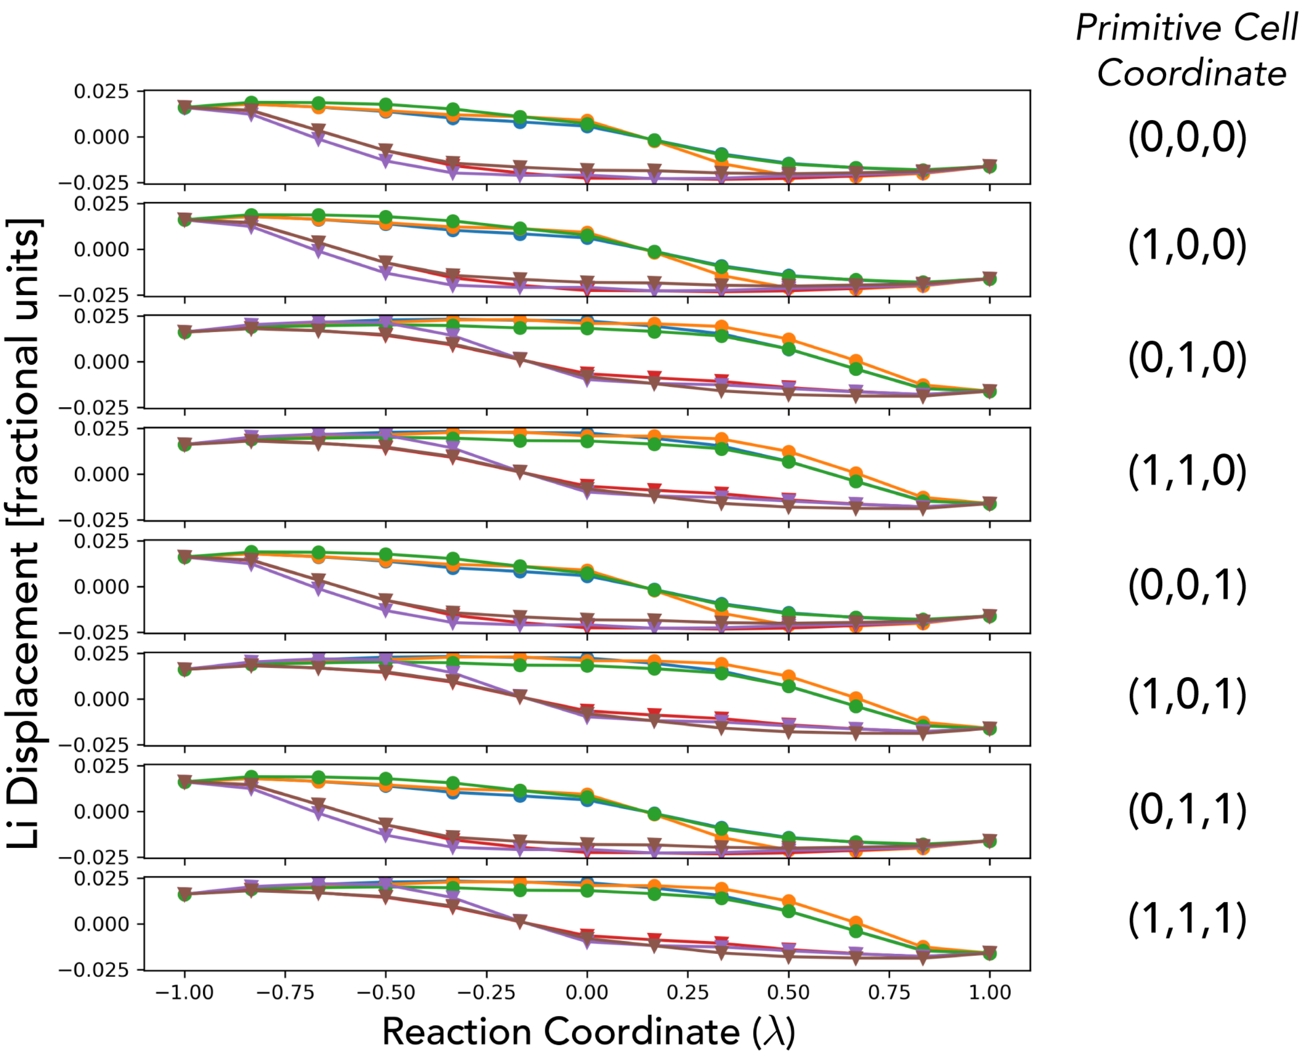


**Supplementary Figure 2.** Plot of the displacement of Li atoms within each primitive rhombohedral unit cell along each of the cell vectors in Fig. 5a as a function of reaction coordinate. Data is plotted for the path with $P\bar{1}$ symmetry shown in purple in Fig. 5b. The high-symmetry structure with $R\bar{3}c$ symmetry is taken as reference. The green, orange, and blue curves correspond to displacements of the Li atom in each primitive cell closest to the origin. The red, purple, and brown curves correspond to displacements along the same directions for the second Li atom in each primitive cell respectively.

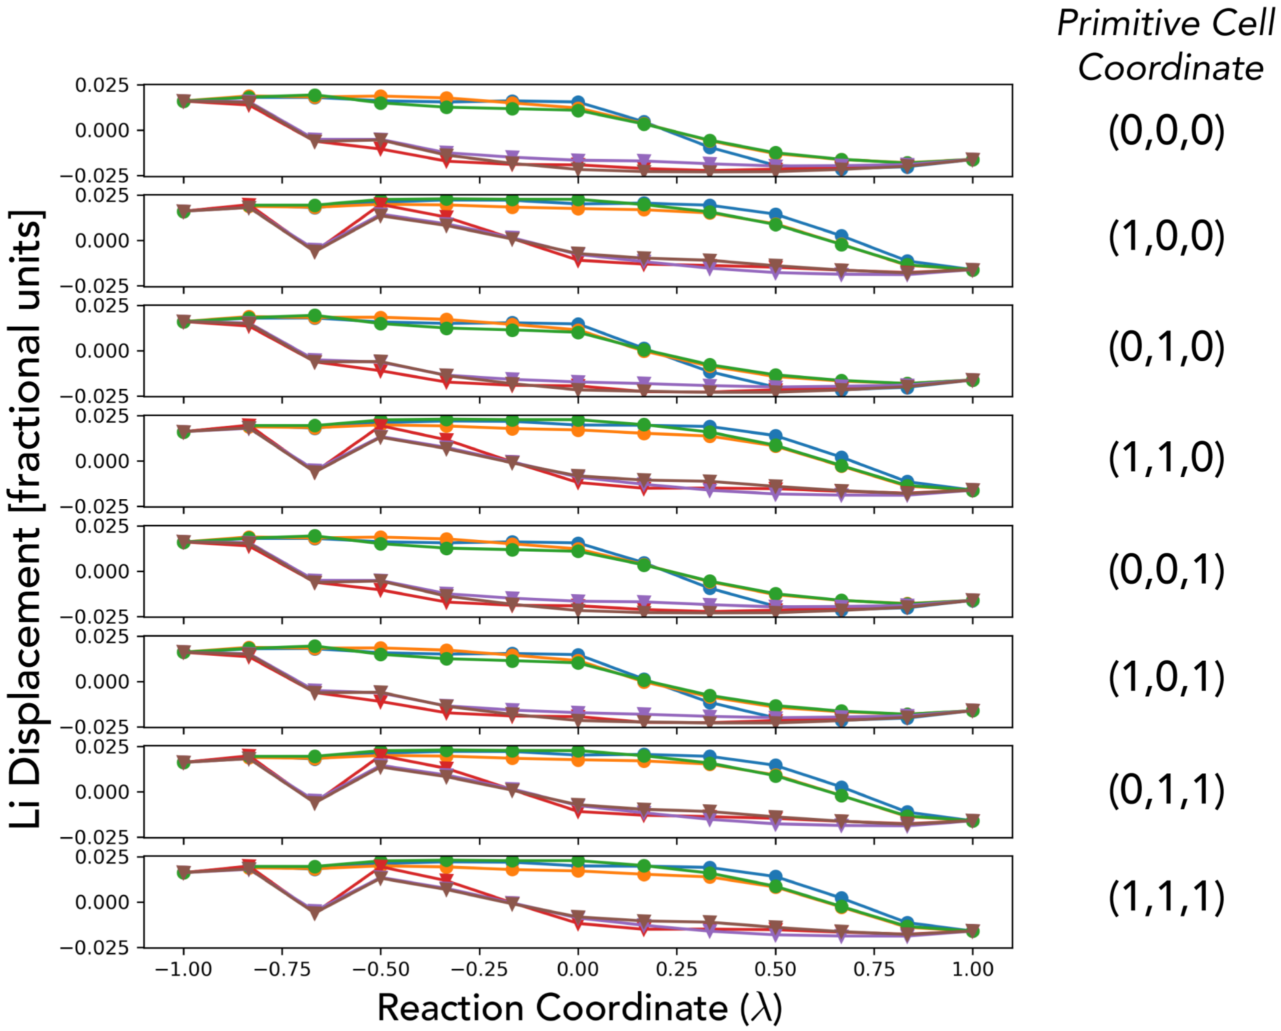


**Supplementary Figure 3.** Plot of the displacement of Li atoms within each primitive rhombohedral unit cell along each of the cell vectors in Fig. 5a as a function of reaction coordinate. Data is plotted for the path with $P1$ symmetry shown in light blue in Fig. 5b. The high-symmetry structure with $R\bar{3}c$ symmetry is taken as reference. The green, orange, and blue curves correspond to displacements of the Li atom in each primitive cell closest to the origin. The red, purple, and brown curves correspond to displacements along the same directions for the second Li atom in each primitive cell respectively.

[1] C. J. Bradley and A. P. Cracknell, *The Mathematical Theory of Symmetry in Solids* (Oxford University Press, Incorporated, 2009).

[2] H. T. Stokes, B. J. Campbell, and R. Cordes, Acta Crystallographica Section A Foundations of Crystallography **69**, 388 (2013).
